# Supplementary material for: Stochastic SketchRefine: Scaling In-Database Decision-Making under Uncertainty to Millions of Tuples
Source: arXiv:2411.17915 source file (2025-04-01)
Supplement: Supplementary file 1 [file quality.tex]

\begin{table}[htb]
\caption{Quality of Generated Packages With Additional CVaR constraints}
\label{tab:cvar_constraint_specified}
\begin{tabular}{@{}llll@{}}
\toprule
                           &    & Rel. Diff. of CVaR (\%) & Rel. Diff. of Obj. Value (\%) \\ \midrule
\multirow{5}{*}{TPC-H}     & Q1 & 10.75                   & -5.34                         \\
                           & Q2 & 10.28                   & -4.24                         \\
                           & Q3 & 10.45                   & -2.36                         \\
                           & Q4 & 10.12                   & -8.91                         \\
                           & Q5 & 10.05                   & -12.31                        \\
\multirow{5}{*}{Portfolio} & Q1 & 10.04                   & -3.43                         \\
                           & Q2 & 10.13                   & -4.15                         \\
                           & Q3 & 10.25                   & -3.91                         \\
                           & Q4 & 10.14                   & -7.81                         \\
                           & Q5 & 10.34                   & -9.46                         \\ \cmidrule(l){2-4} 
\end{tabular}
\end{table}
